# Supplementary material for: DiffEditor: Boosting Accuracy and Flexibility on Diffusion-based Image Editing
Source: arXiv:2402.02583 source file (2024-02-04)
Supplement: Supplementary file 1 [file X_suppl.tex]

% \clearpage
% \setcounter{page}{1}
% \maketitlesupplementary

\section{Rationale}
% \label{sec:rationale}
% 
Having the supplementary compiled together with the main paper means that:
